# Supplementary material for: Integer-Only Neural Network Quantization Scheme Based on Shift-Batch-Normalization
Source: arXiv:2106.00127 source file (2021-05-28)
Supplement: Supplementary file 1 [file appendix.tex]

\appendix
\label{appendix:appendix}
